# Supplementary material for: Geometric flows and the Swampland
Source: arXiv:2307.08320 source file (2023-07-17)
Supplement: Supplementary file 1 [file KKgeneral.tex]

In the following discussion, we will start from a $\left(d+1\right)$-dimensional general relativistic gravitational theory, defined on a Lorentzian manifold $\mathcal{M}$ parametrised by coordinates $x^M$, with the useful notation choice:
\begin{equation}
    x=\left(x^0,\dots,x^{d-1},\lambda\right)\ .
\end{equation}
For the sake of simplicity, we refer to the first $d$ coordinates with the notation $x^\mu$. The action for the $\left(d+1\right)$-dimensional metric tensor $G_{MN}$ is:
\begin{equation}
    S=\frac{1}{\kappa_{d+1}^2}\int_{\mathcal{M}}\diff^{d}x\diff\lambda\sqrt{-G}R_G\ .
\end{equation}
Now, we introduce the metric decomposition
\begin{equation}
    G_{MN} \equiv \begin{pmatrix}
 g_{\mu\nu} & 0\\
 0 & \varphi\end{pmatrix}\ ,
\end{equation}
in which we have used a $d$-dimensional Lorentzian metric $g_{\mu\nu}$ and a scalar $\varphi$ on the $\left(d+1\right)$-dimensional space-time. This is by no means a general ansatz, since we have set the vector component of the metric to zero, but will be enough for our derivation. In particular, we have assumed
\begin{equation}
    \mathcal{M}=\mathcal{N}\times\mathcal{I}\ ,
\end{equation}
in which $\mathcal{N}$ is the $d$-dimensional manifold parametrised by $x^\mu$ and $\mathcal{I}$ is the $1$-dimensional manifold on which $\lambda$ is defined. The inverse metric is:
\begin{equation}
    G^{MN} \equiv \begin{pmatrix}
 g^{\mu\nu} & 0 \\
 0 &  1/\varphi
\end{pmatrix}.
\end{equation}
Now, we have to write down the decomposed form of the metric determinant $G$ and the Ricci scalar $R_G$. The Christoffel symbols $\Gamma^{M}_{NP}$ decompose as follows:
\begin{equation}
    \begin{split}
        2\Gamma^{N}_{PQ}&=G^{N\mu}\left(G_{P\mu,Q}+G_{Q\mu,P}-G_{PQ,\mu}\right)\\
        &\quad+G^{Nd}\left(G_{Pd,Q}+G_{Qd,P}-G_{PQ,d}\right)\ .
    \end{split}
\end{equation}
Focusing on the various specific indices choices, we have:
\begin{equation}
    \begin{split}
        2\Gamma^{\nu}_{\alpha\beta}&=g^{\nu\mu}\left(g_{\alpha\mu,\beta}+g_{\alpha\mu,\beta}-g_{\alpha\beta,\mu}\right)\ ,\quad 
        2\Gamma^{d}_{dd}=\de_d\log{\varphi}\ ,\quad 2\Gamma^{\nu}_{dd}=-\de^\nu\varphi\ ,\\
        2\Gamma^{d}_{\alpha\beta}&=-\varphi^{-1}g_{\alpha\beta,d}\ ,\quad 
        2\Gamma^{\nu}_{\alpha d}=g^{\nu\mu}g_{\alpha\mu,d}\ ,\quad 2\Gamma^{d}_{d\mu}=\de_\mu\log{\varphi}\ .
    \end{split}
\end{equation}
Concerning the Ricci tensor, we get:
\begin{equation}
    R_{MN}= \partial_P\Gamma_{MN}^P - \partial_N\Gamma_{PM}^P + \Gamma_{PQ}^P\Gamma_{MN}^Q - \Gamma_{MQ}^P\Gamma_{PN}^Q\ .
\end{equation}
Referring to the Ricci tensor and covariant derivative on $\mathcal{N}$ as $\Tilde{R}_{\mu\nu}$ and $\tilde{\nabla}$, we obtain:
\begin{equation}
    \begin{split}
        2R_{\mu\nu}&=2\Tilde{R}_{\mu\nu}- \Tilde{\nabla}_\mu\Tilde{\nabla}_\nu\log{\varphi}
 +\frac{1}{\varphi}g_{\mu\nu,d}\partial_d\log{\varphi}
-\frac{1}{2\varphi}g_{\mu\nu,d}\left(\de_d\log{\varphi}+g^{\alpha\rho}g_{\alpha\rho,d}\right)\\
        &\quad+\frac{1}{\varphi} g^{\alpha\rho}g_{\mu\alpha,d} g_{\nu\rho,d}-\frac{1}{\varphi}\de_dg_{\alpha\beta,d}- \frac{1}{2}\de_\mu\log{\varphi}\de_\nu\log{\varphi}\ ,\\
        2R_{dd}&=-\Tilde{\nabla}^2\varphi+\frac{1}{2\varphi}\left(\de_\alpha\varphi\de^\alpha\varphi+g^{\alpha\mu}g_{\alpha\mu,d}\de_d\varphi\right)\\
        &\quad- \partial_d \left(g^{\alpha\mu}g_{\alpha\mu,d}\right)- \frac{1}{2}g^{\alpha\nu}g^{\beta\mu}g_{\beta\nu,d}g_{\alpha\mu,d}\ ,\\
        2R_{d\nu}&=\partial_\alpha\left(g^{\alpha\mu}g_{\nu\mu,d}\right)- \partial_\nu \left(g^{\alpha\mu}g_{\alpha\mu,d}\right)+ \Gamma_{\alpha\beta}^\alpha g^{\beta\mu}g_{\nu\mu,d}- \Gamma_{\alpha\nu}^\beta g^{\alpha\mu}g_{\beta\mu,d}\\
        &\quad+ \frac{1}{2}g^{\alpha\mu}g_{\alpha\mu,d}\de_\nu\log{\varphi}-\frac{1}{2}\de^\alpha\log{\varphi}g_{\alpha\nu,d}\ .
    \end{split}
\end{equation}
Now, we assume the $d$-dimensional metric $g_{\mu\nu}$ to evolve according to Ricci flow along $\lambda$:
\begin{equation}
    g_{\mu\nu,d}=-2\Tilde{R}_{\mu\nu}\ .
\end{equation}
Hence, we get:
\begin{equation}
    \begin{split}
        2R_{\mu\nu}&=2\Tilde{R}_{\mu\nu}- \Tilde{\nabla}_\mu\Tilde{\nabla}_\nu\log{\varphi}
 -\frac{2}{\varphi}\Tilde{R}_{\mu\nu}\partial_d\log{\varphi}
+\frac{1}{\varphi}\Tilde{R}_{\mu\nu}\left(\de_d\log{\varphi}-2\Tilde{R}\right)\\
        &\quad+\frac{4}{\varphi} g^{\alpha\rho}\Tilde{R}_{\mu\alpha} \Tilde{R}_{\nu\rho}+\frac{2}{\varphi}\de_d\Tilde{R}_{\mu\nu}- \frac{1}{2}\de_\mu\log{\varphi}\de_\nu\log{\varphi}\ ,\\
        2R_{dd}&=-\Tilde{\nabla}^2\varphi+\frac{1}{2\varphi}\left(\de_\alpha\varphi\de^\alpha\varphi-2\Tilde{R}\de_d\varphi\right)+2 \partial_d \Tilde{R}-2\Tilde{R}^{\alpha\mu}\Tilde{R}_{\alpha\mu}\ ,\\
        2R_{d\nu}&=2 \partial_\nu\Tilde{R}-2\nabla_\alpha\Tilde{R}^{\alpha}{}_\nu-\Tilde{R}\de_\nu\log{\varphi}+\Tilde{R}_{\nu\alpha}\de^\alpha\log{\varphi}\ .
    \end{split}
\end{equation}
The Ricci scalar is simply given by:
\begin{equation}
    \begin{split}
        2R&=2g^{\mu\nu}R_{\mu\nu}+2\varphi^{-1}R_{dd}\\
        &=2\Tilde{R}- \Tilde{\nabla}^2\log{\varphi}
-\frac{1}{\varphi}\Tilde{R}\left(\de_d\log{\varphi}+2\Tilde{R}\right)\\
        &\quad+\frac{2}{\varphi} \Tilde{R}^{\mu\alpha} \Tilde{R}_{\mu\alpha}+\frac{2}{\varphi}g^{\mu\nu}\de_d\Tilde{R}_{\mu\nu}- \frac{1}{2}\de^\mu\log{\varphi}\de_\mu\log{\varphi}\\
        &\quad-\varphi^{-1}\Tilde{\nabla}^2\varphi+\frac{1}{2\varphi^2}\left(\de_\alpha\varphi\de^\alpha\varphi-2\Tilde{R}\de_d\varphi\right)+2 \varphi^{-1}\partial_d \Tilde{R}\ .
    \end{split}
\end{equation}
If we assume $\varphi=1$, we obtain:
\begin{equation}
    \begin{split}
        R_{\mu\nu}&=\Tilde{R}_{\mu\nu}-\Tilde{R}\Tilde{R}_{\mu\nu}+2g^{\alpha\rho}\Tilde{R}_{\mu\alpha} \Tilde{R}_{\nu\rho}+\de_d\Tilde{R}_{\mu\nu}\ ,\\
        R_{dd}&= \partial_d \Tilde{R}-\Tilde{R}^{\alpha\mu}\Tilde{R}_{\alpha\mu}\ ,\\
        R_{d\nu}&=2 \partial_\nu\Tilde{R}-\nabla_\alpha\Tilde{R}^{\alpha}{}_\nu\ ,\\
        R&=\Tilde{R}-\Tilde{R}^2+\Tilde{R}^{\mu\alpha} \Tilde{R}_{\mu\alpha}+g^{\mu\nu}\de_d\Tilde{R}_{\mu\nu}+\partial_d \Tilde{R}\ .
    \end{split}
\end{equation}
Starting from the $\left(d+1\right)$-dimensional Einstein field equations
\begin{equation}
    2R_{MN}=G_{MN}R\ ,
\end{equation}
we obtain the various components:
\begin{equation}
    \begin{split}
        \Tilde{R}_{\mu\nu}-\Tilde{R}\Tilde{R}_{\mu\nu}+2g^{\alpha\rho}\Tilde{R}_{\mu\alpha} \Tilde{R}_{\nu\rho}+\de_d\Tilde{R}_{\mu\nu}&=\frac{1}{2}g_{\mu\nu}\left(\Tilde{R}-\Tilde{R}^2+\Tilde{R}^{\mu\alpha} \Tilde{R}_{\mu\alpha}+g^{\mu\nu}\de_d\Tilde{R}_{\mu\nu}+\partial_d \Tilde{R}\right)\\
        \partial_d \Tilde{R}-\Tilde{R}^{\alpha\mu}\Tilde{R}_{\alpha\mu}&=\frac{1}{2}\left(\Tilde{R}-\Tilde{R}^2+\Tilde{R}^{\mu\alpha} \Tilde{R}_{\mu\alpha}+g^{\mu\nu}\de_d\Tilde{R}_{\mu\nu}+\partial_d \Tilde{R}\right) \\
        2 \partial_\nu\Tilde{R}-\nabla_\alpha\Tilde{R}^{\alpha}{}_\nu&=0\ .
    \end{split}
\end{equation}
The last one is simply the Bianchi identity in $d$ dimensions. Combining the first and the second one, we get:
\begin{equation}
    \Tilde{R}_{\mu\nu}-\Tilde{R}\Tilde{R}_{\mu\nu}+2g^{\alpha\rho}\Tilde{R}_{\mu\alpha} \Tilde{R}_{\nu\rho}+\de_d\Tilde{R}_{\mu\nu}=g_{\mu\nu}\left(\partial_d \Tilde{R}-\Tilde{R}^{\alpha\mu}\Tilde{R}_{\alpha\mu}\right)
\end{equation}
Contracting with $g^{\mu\nu}$:
\begin{equation}
    \Tilde{R}-\Tilde{R}^2+(2+d)\Tilde{R}^{\mu\nu} \Tilde{R}_{\mu\nu}+g^{\mu\nu}\de_d\Tilde{R}_{\mu\nu}=d\partial_d \Tilde{R}
\end{equation}
